# Supplementary material for: Large Vibrationally Induced Parity Violation Effects in CHDBrI$^+$ $-$ A Promising Candidate for Future Experiments
Source: arXiv:2306.09763 source file (2023-08-08)
Supplement: Supplementary file 1 [file SI.pdf]

# Supporting Information:

## Large Vibrationally Induced Parity Violation Effects in $\text{CHDBrI}^+$ – A Promising Candidate for Future Experiments

Eduardus Eduardus,<sup>†</sup> Yuval Shagam,<sup>‡</sup> Arie Landau,<sup>¶</sup> Shirin Faraji,<sup>§</sup> Peter Schwerdtfeger,<sup>||</sup> Anastasia Borschevsky,<sup>†</sup> and Lukáš F. Pašteka<sup>\*,†,⊥</sup>

<sup>†</sup>*Van Swinderen Institute for Particle Physics and Gravity (VSI), University of Groningen, Groningen, The Netherlands*

<sup>‡</sup>*Schulich Faculty of Chemistry, Solid State Institute and The Helen Diller Quantum Center, Technion-Israel Institute of Technology, Haifa 32000, Israel*

<sup>¶</sup>*Schulich Faculty of Chemistry, The Helen Diller Quantum Center and The Institute of Advanced Studies in Theoretical Chemistry, Technion-Israel Institute of Technology, Haifa 32000, Israel*

<sup>§</sup>*Zernike Institute for Advanced Materials, Faculty of Science and Engineering, University of Groningen, Nijenborgh 4, 9747AG Groningen The Netherlands*

<sup>||</sup>*Centre for Theoretical Chemistry and Physics, The New Zealand Institute for Advanced Study, Massey University Auckland, Private Bag 102904, 0632 Auckland, New Zealand*

<sup>⊥</sup>*Department of Physical and Theoretical Chemistry, Faculty of Natural Sciences, Comenius University, Mlynská dolina, 84215 Bratislava, Slovakia*

E-mail: l.f.pasteka@rug.nl

In this supporting information, we provide additional data for the geometries, vibrational harmonic and anharmonic treatment of  $\text{CH}_2\text{BrI}$ ,  $\text{CHDBrI}$ ,  $\text{CH}_2\text{BrI}^+$  and  $\text{CHDBrI}^+$  using vibrational perturbation theory<sup>1-4</sup> and a few selected density functionals, as well as for parity violation (PV) contributions calculated using the CAMB3LYP\* functional,<sup>5</sup> as described in the main text. Data in Sections S1 – S3 are presented in order to validate the used methodology with respect to different levels of theory as well as experimental data available for  $\text{CH}_2\text{BrI}$ . Data in Sections S4 and S5 are presented as further analysis of the parity violation effects in  $\text{CH}_2\text{BrI}^+$  and  $\text{CHDBrI}^+$ .

Calculations using the PBE, PB86, B3LYP and  $\omega\text{B97X-D}$  functionals were performed in Gaussian 16. CCSD(T) calculations were performed in Molpro 2021.2.0.

## S1. Geometries

Table S1 summarizes the optimized bond distances and angles for  $\text{CH}_2\text{BrI}$  and  $\text{CH}_2\text{BrI}^+$  and dipole moments for  $\text{CH}_2\text{BrI}$ , obtained with different DFT functionals and the Def2-QZVPPD basis set.<sup>6</sup> We have also performed geometry optimization using the coupled cluster approach with single, double, and perturbative triple excitations (CCSD(T)) with 40 (39) correlated electrons (corresponding to the frozen core approximation up to  $-5$  a.u.). As can be seen, the  $\omega\text{B97M-V}$  functional<sup>7</sup> bond lengths and angles are in excellent agreement with the results obtained using CCSD(T) and also compare well to the experimentally derived  $r_0$ -structural parameters of  $\text{CH}_2\text{BrI}$ .<sup>8</sup>

We note that for the positively charged species care has to be taken as the geometry optimization may lead to a minimum with the hole, caused by the removal of an electron, being artificially localized at the iodine atom. This state lies 0.0123 a.u. (32 kJ/mol) above the global minimum where the hole is partially delocalized over both halogen atoms. This artificial localization leads to unreasonable values for the vibrational spectrum and intensities in the lower frequency range and should therefore to be avoided.

Table S1: Equilibrium bond lengths  $r_e$  (in Å), bond angles  $\alpha$  (in degrees), and dipole moments (in Debye, neutral molecule only) for CH<sub>2</sub>BrI and CH<sub>2</sub>BrI<sup>+</sup> obtained from various DFT and CCSD(T) calculations and compared to experimentally derived parameters.<sup>8</sup>

| Molecule                         | Property         | PBE   | PB86  | B3LYP | $\omega$ B97X-D | $\omega$ B97M-V | CCSD(T) | Exp. <sup>a</sup> |
|----------------------------------|------------------|-------|-------|-------|-----------------|-----------------|---------|-------------------|
| CH <sub>2</sub> BrI              | $r_e$ (CH)       | 1.090 | 1.089 | 1.080 | 1.081           | 1.080           | 1.082   | (1.083)           |
|                                  | $r_e$ (CBr)      | 1.940 | 1.946 | 1.943 | 1.926           | 1.923           | 1.923   | 1.926             |
|                                  | $r_e$ (CI)       | 2.150 | 2.156 | 2.150 | 2.125           | 2.121           | 2.123   | (2.131)           |
|                                  | $\alpha$ (HCH)   | 112.4 | 112.5 | 112.2 | 111.4           | 111.5           | 111.9   | 107.7             |
|                                  | $\alpha$ (HCBBr) | 107.8 | 107.8 | 107.7 | 107.9           | 108.0           | 108.0   | 107.3             |
|                                  | $\alpha$ (HCl)   | 107.0 | 107.0 | 107.1 | 107.6           | 107.7           | 107.5   | –                 |
|                                  | $\alpha$ (BrCI)  | 114.9 | 114.9 | 114.9 | 114.6           | 113.9           | 113.9   | 113.5             |
|                                  | $\mu_e$          | 1.262 | 1.277 | 1.309 | 1.327           | 1.321           | 1.318   | –                 |
| CH <sub>2</sub> BrI <sup>+</sup> | $r_e$ (CH)       | 1.091 | 1.091 | 1.081 | 1.082           | 1.080           | 1.084   | –                 |
|                                  | $r_e$ (CBr)      | 1.939 | 1.944 | 1.937 | 1.921           | 1.917           | 1.922   | –                 |
|                                  | $r_e$ (CI)       | 2.143 | 2.151 | 2.146 | 2.118           | 2.115           | 2.120   | –                 |
|                                  | $\alpha$ (HCH)   | 116.4 | 116.5 | 116.1 | 115.6           | 115.6           | 116.5   | –                 |
|                                  | $\alpha$ (HCBBr) | 111.1 | 111.0 | 111.1 | 111.4           | 111.9           | 111.4   | –                 |
|                                  | $\alpha$ (HCl)   | 110.8 | 110.7 | 110.6 | 111.3           | 110.7           | 111.0   | –                 |
|                                  | $\alpha$ (BrCI)  | 94.5  | 94.8  | 95.4  | 93.7            | 94.1            | 93.1    | –                 |

<sup>a</sup>  $r_0$ -structure derived from isotopic substitution rotational spectra. Numbers in parentheses were fixed to *ab initio* data in the fitting procedure.

## S2. Vibrational Analysis

Tables S2 to S5 summarize the calculated harmonic and anharmonic vibrational frequencies, intensities and lifetimes for the different molecules at different levels of density functional theory using vibrational perturbation theory. Modes 1 to 7 are fairly harmonic in their nature (see Figure S3) and thus the harmonic approximation introduces only a relatively small error in vibrational frequencies compared to the anharmonic results ( $< 40 \text{ cm}^{-1}$ ). The C–H/D stretching modes 8 and 9 are the most anharmonic and the error of the harmonic approximation is also the largest ( $100 - 200 \text{ cm}^{-1}$ ). For CH<sub>2</sub>BrI the smallest root mean square deviation from experiment<sup>9,10</sup> is obtained for the B3LYP and  $\omega$ B97M-V functionals.<sup>7</sup>

Table S2: Vibrational harmonic (harm) and anharmonic (anharm) fundamental transition frequencies (in  $\text{cm}^{-1}$ ) for the molecules  $\text{CH}_2\text{BrI}$ ,  $\text{CH}_2\text{BrI}^+$ ,  $\text{CHDBrI}$ , and  $\text{CHDBrI}^+$  obtained from a 3-mode analysis.

| Mode                      | PBE<br>harm | PBE<br>anharm | PB86<br>harm | PB86<br>anharm | B3LYP<br>harm | B3LYP<br>anharm | $\omega\text{B97X-D}$<br>harm | $\omega\text{B97X-D}$<br>anharm | $\omega\text{B97M-V}$<br>harm | $\omega\text{B97M-V}$<br>anharm | Exp. <sup>9,10</sup> |
|---------------------------|-------------|---------------|--------------|----------------|---------------|-----------------|-------------------------------|---------------------------------|-------------------------------|---------------------------------|----------------------|
| $\text{CH}_2\text{BrI}$   |             |               |              |                |               |                 |                               |                                 |                               |                                 |                      |
| 1                         | 136.3       | 136.0         | 135.3        | 136.6          | 140.2         | 143.3           | 145.9                         | 143.0                           | 146.4                         | 144.9                           | 144                  |
| 2                         | 508.9       | 499.7         | 503.1        | 493.2          | 515.1         | 505.3           | 545.0                         | 535.0                           | 548.4                         | 540.8                           | 517                  |
| 3                         | 599.2       | 582.3         | 588.6        | 572.6          | 608.2         | 593.4           | 663.2                         | 644.2                           | 671.2                         | 652.9                           | 616                  |
| 4                         | 739.2       | 732.4         | 738.9        | 732.3          | 764.6         | 757.7           | 775.3                         | 767.5                           | 774.5                         | 763.4                           | 754                  |
| 5                         | 1047.6      | 1030.0        | 1046.9       | 1028.1         | 1089.4        | 1072.2          | 1112.0                        | 1078.4                          | 1107.4                        | 1087.6                          | 1065                 |
| 6                         | 1126.4      | 1106.8        | 1127.5       | 1107.8         | 1178.3        | 1159.3          | 1200.1                        | 1163.1                          | 1191.9                        | 1168.1                          | 1150                 |
| 7                         | 1368.3      | 1328.7        | 1370.0       | 1329.3         | 1426.0        | 1386.0          | 1441.5                        | 1402.6                          | 1433.9                        | 1369.7                          | 1374                 |
| 8                         | 3059.5      | 2933.7        | 3052.6       | 2924.6         | 3133.4        | 3009.7          | 3148.4                        | 2957.4                          | 3151.2                        | 3019.3                          | 2978                 |
| 9                         | 3147.9      | 3002.0        | 3141.8       | 2994.4         | 3220.8        | 3077.0          | 3233.6                        | 3021.3                          | 3232.6                        | 3083.5                          | 3091                 |
| RMSD                      | 37.7        | 42.6          | 35.7         | 46.6           | 72.9          | 17.4            | 84.9                          | 28.9                            | 84.6                          | 24.4                            |                      |
| $\text{CH}_2\text{BrI}^+$ |             |               |              |                |               |                 |                               |                                 |                               |                                 |                      |
| 1                         | 135.6       | 134.9         | 133.9        | 138.7          | 137.0         | 128.4           | 153.3                         | 159.9                           | 152.3                         |                                 |                      |
| 2                         | 515.3       | 493.3         | 505.3        | 485.0          | 509.4         | 487.9           | 551.0                         | 535.8                           | 538.5                         |                                 |                      |
| 3                         | 603.2       | 585.3         | 594.1        | 582.9          | 605.8         | 589.2           | 645.7                         | 637.4                           | 651.0                         |                                 |                      |
| 4                         | 794.3       | 790.9         | 793.9        | 788.5          | 821.9         | 813.6           | 837.4                         | 827.5                           | 835.3                         |                                 |                      |
| 5                         | 981.9       | 963.0         | 981.8        | 965.5          | 1020.9        | 997.9           | 1033.9                        | 1029.6                          | 1028.7                        |                                 |                      |
| 6                         | 1095.3      | 1073.9        | 1096.7       | 1079.1         | 1140.7        | 1119.3          | 1154.5                        | 1146.9                          | 1143.9                        |                                 |                      |
| 7                         | 1361.5      | 1324.4        | 1363.4       | 1327.2         | 1417.5        | 1378.0          | 1431.7                        | 1396.0                          | 1422.5                        |                                 |                      |
| 8                         | 3054.6      | 2930.8        | 3048.0       | 2925.0         | 3129.8        | 3008.3          | 3145.6                        | 3000.3                          | 3150.9                        |                                 |                      |
| 9                         | 3168.1      | 3027.9        | 3162.6       | 3020.5         | 3242.2        | 3101.4          | 3256.8                        | 3089.5                          | 3259.7                        |                                 |                      |
| $\text{CHDBrI}$           |             |               |              |                |               |                 |                               |                                 |                               |                                 |                      |
| 1                         | 136.0       | 128.6         | 135.0        | 129.4          | 139.9         | 139.8           | 145.6                         | 130.9                           | 146.3                         |                                 |                      |
| 2                         | 492.0       | 478.5         | 486.6        | 476.5          | 498.1         | 488.2           | 525.6                         | 513.5                           | 539.5                         |                                 |                      |
| 3                         | 583.8       | 564.9         | 574.1        | 558.0          | 592.8         | 577.1           | 641.0                         | 618.7                           | 644.6                         |                                 |                      |
| 4                         | 636.9       | 627.4         | 636.2        | 629.1          | 658.0         | 650.9           | 669.3                         | 658.2                           | 679.2                         |                                 |                      |
| 5                         | 790.8       | 771.4         | 789.8        | 774.4          | 823.8         | 809.4           | 847.0                         | 817.9                           | 845.1                         |                                 |                      |
| 6                         | 1090.1      | 1064.2        | 1090.6       | 1067.7         | 1138.3        | 1117.6          | 1161.1                        | 1117.0                          | 1155.6                        |                                 |                      |
| 7                         | 1217.3      | 1183.2        | 1218.8       | 1185.8         | 1268.3        | 1235.1          | 1281.8                        | 1248.4                          | 1283.9                        |                                 |                      |
| 8                         | 2276.5      | 2202.1        | 2271.7       | 2197.5         | 2330.7        | 2259.6          | 2341.2                        | 2237.2                          | 2345.8                        |                                 |                      |
| 9                         | 3106.8      | 2965.8        | 3100.3       | 2958.0         | 3180.1        | 3042.5          | 3193.8                        | 2989.1                          | 3198.0                        |                                 |                      |
| $\text{CHDBrI}^+$         |             |               |              |                |               |                 |                               |                                 |                               |                                 |                      |
| 1                         | 135.4       | 136.1         | 133.7        | 128.3          | 136.8         | 130.9           | 153.1                         | 149.0                           | 149.1                         |                                 |                      |
| 2                         | 499.1       | 481.4         | 490.2        | 471.0          | 494.9         | 476.6           | 532.3                         | 517.5                           | 524.4                         |                                 |                      |
| 3                         | 582.4       | 570.7         | 574.4        | 560.4          | 585.9         | 572.2           | 620.6                         | 607.2                           | 619.8                         |                                 |                      |
| 4                         | 674.2       | 668.8         | 673.0        | 663.8          | 696.7         | 689.6           | 713.8                         | 702.5                           | 709.9                         |                                 |                      |
| 5                         | 755.9       | 744.5         | 755.0        | 738.3          | 783.7         | 769.1           | 797.1                         | 787.6                           | 796.5                         |                                 |                      |
| 6                         | 1047.3      | 1029.8        | 1048.1       | 1026.6         | 1090.2        | 1073.2          | 1104.8                        | 1091.4                          | 1103.8                        |                                 |                      |
| 7                         | 1216.2      | 1188.0        | 1217.8       | 1185.7         | 1265.9        | 1233.3          | 1279.0                        | 1247.0                          | 1274.9                        |                                 |                      |
| 8                         | 2281.5      | 2211.5        | 2277.0       | 2204.2         | 2336.7        | 2266.3          | 2348.4                        | 2263.2                          | 2354.0                        |                                 |                      |
| 9                         | 3116.3      | 2982.6        | 3110.3       | 2973.2         | 3190.8        | 3057.3          | 3205.9                        | 3044.9                          | 3213.8                        |                                 |                      |

Table S3: Harmonic (harm) and anharmonic (anharm) IR intensities (in km/mol) for the fundamental transitions of the molecules CH<sub>2</sub>BrI, CH<sub>2</sub>BrI<sup>+</sup>, CHDBrI, and CHDBrI<sup>+</sup> obtained from a 3-mode analysis.

| Mode                             | PBE<br>harm | PBE<br>anharm | PB86<br>harm | PB86<br>anharm | B3LYP<br>harm | B3LYP<br>anharm | $\omega$ B97X-D<br>harm | $\omega$ B97X-D<br>anharm | $\omega$ B97M-V<br>harm |
|----------------------------------|-------------|---------------|--------------|----------------|---------------|-----------------|-------------------------|---------------------------|-------------------------|
| CH <sub>2</sub> BrI              |             |               |              |                |               |                 |                         |                           |                         |
| 1                                | 0.041       | 0.039         | 0.040        | 0.038          | 0.059         | 0.057           | 0.110                   | 0.108                     | 0.105                   |
| 2                                | 8.984       | 11.510        | 10.473       | 13.226         | 6.547         | 8.337           | 2.372                   | 2.552                     | 2.873                   |
| 3                                | 83.097      | 84.491        | 86.608       | 87.923         | 78.170        | 80.713          | 57.181                  | 60.437                    | 54.843                  |
| 4                                | 5.027       | 4.809         | 4.902        | 4.680          | 4.900         | 4.722           | 5.114                   | 4.956                     | 4.636                   |
| 5                                | 0.021       | 0.071         | 0.017        | 0.034          | 0.009         | 0.024           | 0.005                   | 0.012                     | 0.003                   |
| 6                                | 69.195      | 61.932        | 72.708       | 65.203         | 81.769        | 74.460          | 73.784                  | 58.873                    | 74.952                  |
| 7                                | 0.002       | 0.026         | 0.024        | 0.037          | 0.034         | 0.051           | 0.032                   | 0.035                     | 0.006                   |
| 8                                | 0.367       | 1.102         | 0.435        | 1.282          | 0.409         | 1.202           | 0.478                   | 0.940                     | 0.821                   |
| 9                                | 4.110       | 1.964         | 3.691        | 1.682          | 3.957         | 1.915           | 3.919                   | 2.406                     | 3.249                   |
| CH <sub>2</sub> BrI <sup>+</sup> |             |               |              |                |               |                 |                         |                           |                         |
| 1                                | 0.457       | 0.433         | 0.420        | 0.395          | 0.874         | 0.834           | 1.963                   | 1.860                     | 3.410                   |
| 2                                | 13.617      | 13.988        | 14.279       | 15.330         | 17.277        | 18.359          | 20.046                  | 21.082                    | 25.556                  |
| 3                                | 7.084       | 7.140         | 7.563        | 7.944          | 7.540         | 7.980           | 7.024                   | 7.345                     | 7.240                   |
| 4                                | 2.400       | 2.296         | 2.316        | 2.196          | 2.364         | 2.275           | 2.599                   | 2.643                     | 2.224                   |
| 5                                | 0.023       | 0.003         | 0.020        | 0.041          | 0.021         | 0.018           | 0.017                   | 0.067                     | 0.037                   |
| 6                                | 1.168       | 0.852         | 1.298        | 1.037          | 1.071         | 0.902           | 0.947                   | 0.886                     | 1.044                   |
| 7                                | 0.472       | 0.502         | 0.485        | 0.467          | 0.769         | 0.737           | 0.780                   | 0.844                     | 1.273                   |
| 8                                | 15.139      | 13.982        | 14.298       | 12.129         | 13.878        | 12.050          | 14.524                  | 13.164                    | 13.156                  |
| 9                                | 28.178      | 25.571        | 27.222       | 22.979         | 27.985        | 24.190          | 29.027                  | 25.828                    | 28.327                  |
| CHDBrI                           |             |               |              |                |               |                 |                         |                           |                         |
| 1                                | 0.042       | 0.039         | 0.041        | 0.039          | 0.060         | 0.059           | 0.110                   | 0.109                     | 0.066                   |
| 2                                | 6.855       | 7.705         | 8.020        | 9.483          | 5.078         | 6.063           | 1.865                   | 1.820                     | 1.547                   |
| 3                                | 67.849      | 68.891        | 72.167       | 74.428         | 63.683        | 66.744          | 40.530                  | 41.530                    | 37.709                  |
| 4                                | 2.575       | 2.427         | 2.499        | 2.365          | 2.503         | 2.415           | 2.694                   | 2.510                     | 2.393                   |
| 5                                | 35.292      | 33.735        | 35.548       | 32.982         | 35.912        | 34.211          | 34.834                  | 33.857                    | 35.663                  |
| 6                                | 43.512      | 39.993        | 45.825       | 41.467         | 51.858        | 45.290          | 47.063                  | 39.287                    | 47.343                  |
| 7                                | 1.116       | 0.798         | 1.110        | 0.939          | 1.135         | 1.088           | 1.117                   | 0.781                     | 1.007                   |
| 8                                | 1.044       | 0.936         | 0.981        | 0.950          | 1.031         | 1.074           | 1.048                   | 1.314                     | 1.030                   |
| 9                                | 2.447       | 1.536         | 2.247        | 1.502          | 2.375         | 1.579           | 2.377                   | 1.734                     | 2.125                   |
| CHDBrI <sup>+</sup>              |             |               |              |                |               |                 |                         |                           |                         |
| 1                                | 0.455       | 0.437         | 0.417        | 0.396          | 0.871         | 0.836           | 1.961                   | 1.839                     | 4.373                   |
| 2                                | 11.503      | 12.551        | 12.197       | 13.291         | 15.088        | 16.256          | 17.054                  | 18.310                    | 21.834                  |
| 3                                | 6.143       | 6.557         | 6.598        | 6.952          | 6.680         | 7.007           | 6.079                   | 5.966                     | 6.490                   |
| 4                                | 1.970       | 1.922         | 1.934        | 1.896          | 1.947         | 1.938           | 2.332                   | 2.836                     | 2.284                   |
| 5                                | 1.548       | 1.254         | 1.546        | 1.370          | 1.342         | 1.207           | 1.716                   | 1.485                     | 2.049                   |
| 6                                | 1.034       | 0.811         | 1.149        | 0.856          | 0.955         | 0.762           | 0.795                   | 0.672                     | 0.746                   |
| 7                                | 1.002       | 0.942         | 1.043        | 0.949          | 1.327         | 1.151           | 1.303                   | 1.297                     | 1.790                   |
| 8                                | 8.438       | 7.114         | 7.940        | 6.556          | 7.948         | 6.688           | 8.445                   | 7.412                     | 7.551                   |
| 9                                | 22.438      | 19.055        | 21.539       | 18.010         | 21.754        | 18.461          | 22.602                  | 19.943                    | 20.723                  |

Table S4: Harmonic (harm) and anharmonic (anharm) lifetimes for the fundamental transitions of the molecules  $\text{CH}_2\text{BrI}$ ,  $\text{CH}_2\text{BrI}^+$ ,  $\text{CHDBrI}$ , and  $\text{CHDBrI}^+$  obtained from a 3-mode analysis.

| Mode                      | PBE<br>harm | PBE<br>anharm | PB86<br>harm | PB86<br>anharm | B3LYP<br>harm | B3LYP<br>anharm | $\omega\text{B97X-D}$<br>harm | $\omega\text{B97X-D}$<br>anharm | $\omega\text{B97M-V}$<br>harm |
|---------------------------|-------------|---------------|--------------|----------------|---------------|-----------------|-------------------------------|---------------------------------|-------------------------------|
| $\text{CH}_2\text{BrI}$   |             |               |              |                |               |                 |                               |                                 |                               |
| 1                         | 2.91 h      | 3.08 h        | 3.03 h       | 3.13 h         | 1.91 h        | 1.9 h           | 56.9 min                      | 1.01 h                          | 59.2 min                      |
| 2                         | 3.44 s      | 2.78 s        | 3.02 s       | 2.48 s         | 4.6 s         | 3.75 s          | 11.3 s                        | 10.9 s                          | 9.25 s                        |
| 3                         | 268 ms      | 279 ms        | 266 ms       | 277 ms         | 276 ms        | 281 ms          | 318 ms                        | 319 ms                          | 323 ms                        |
| 4                         | 2.91 s      | 3.1 s         | 2.99 s       | 3.18 s         | 2.79 s        | 2.95 s          | 2.6 s                         | 2.74 s                          | 2.87 s                        |
| 5                         | 5.78 min    | 1.77 min      | 7.15 min     | 3.71 min       | 12.5 min      | 4.83 min        | 21.5 min                      | 9.55 min                        | 36.2 min                      |
| 6                         | 91 ms       | 105 ms        | 86.5 ms      | 99.9 ms        | 70.4 ms       | 79.9 ms         | 75.2 ms                       | 100 ms                          | 75.1 ms                       |
| 7                         | 35.6 min    | 2.9 min       | 2.96 min     | 2.04 min       | 1.93 min      | 1.36 min        | 2 min                         | 1.93 min                        | 10.8 min                      |
| 8                         | 2.33 s      | 843 ms        | 1.97 s       | 729 ms         | 1.99 s        | 734 ms          | 1.69 s                        | 972 ms                          | 980 ms                        |
| 9                         | 196 ms      | 452 ms        | 219 ms       | 530 ms         | 195 ms        | 441 ms          | 195 ms                        | 364 ms                          | 235 ms                        |
| $\text{CH}_2\text{BrI}^+$ |             |               |              |                |               |                 |                               |                                 |                               |
| 1                         | 15.9 min    | 16.9 min      | 17.7 min     | 17.5 min       | 8.12 min      | 9.69 min        | 2.89 min                      | 2.8 min                         | 1.68 min                      |
| 2                         | 2.21 s      | 2.35 s        | 2.19 s       | 2.22 s         | 1.78 s        | 1.83 s          | 1.31 s                        | 1.32 s                          | 1.08 s                        |
| 3                         | 3.1 s       | 3.27 s        | 2.99 s       | 2.96 s         | 2.89 s        | 2.89 s          | 2.73 s                        | 2.68 s                          | 2.6 s                         |
| 4                         | 5.28 s      | 5.57 s        | 5.48 s       | 5.85 s         | 5.01 s        | 5.31 s          | 4.39 s                        | 4.42 s                          | 5.15 s                        |
| 5                         | 6.01 min    | 47.9 min      | 6.91 min     | 3.49 min       | 6.09 min      | 7.43 min        | 7.33 min                      | 1.88 min                        | 3.4 min                       |
| 6                         | 5.7 s       | 8.13 s        | 5.12 s       | 6.62 s         | 5.74 s        | 7.07 s          | 6.33 s                        | 6.86 s                          | 5.85 s                        |
| 7                         | 9.14 s      | 9.08 s        | 8.87 s       | 9.72 s         | 5.17 s        | 5.71 s          | 5 s                           | 4.86 s                          | 3.1 s                         |
| 8                         | 56.6 ms     | 66.6 ms       | 60.2 ms      | 77 ms          | 58.8 ms       | 73.3 ms         | 55.6 ms                       | 67.4 ms                         | 61.2 ms                       |
| 9                         | 28.3 ms     | 34.1 ms       | 29.4 ms      | 38.1 ms        | 27.2 ms       | 34.4 ms         | 26 ms                         | 32.4 ms                         | 26.6 ms                       |
| $\text{CHDBrI}$           |             |               |              |                |               |                 |                               |                                 |                               |
| 1                         | 2.86 h      | 3.44 h        | 2.97 h       | 3.4 h          | 1.89 h        | 1.93 h          | 57.1 min                      | 1.19 h                          | 1.57 h                        |
| 2                         | 4.82 s      | 4.53 s        | 4.21 s       | 3.71 s         | 6.34 s        | 5.53 s          | 15.5 s                        | 16.7 s                          | 17.8 s                        |
| 3                         | 346 ms      | 364 ms        | 336 ms       | 345 ms         | 357 ms        | 360 ms          | 480 ms                        | 503 ms                          | 510 ms                        |
| 4                         | 7.65 s      | 8.37 s        | 7.9 s        | 8.54 s         | 7.38 s        | 7.81 s          | 6.62 s                        | 7.35 s                          | 7.24 s                        |
| 5                         | 362 ms      | 398 ms        | 360 ms       | 404 ms         | 328 ms        | 357 ms          | 320 ms                        | 353 ms                          | 314 ms                        |
| 6                         | 155 ms      | 176 ms        | 147 ms       | 169 ms         | 119 ms        | 141 ms          | 126 ms                        | 163 ms                          | 126 ms                        |
| 7                         | 4.83 s      | 7.15 s        | 4.85 s       | 6.05 s         | 4.38 s        | 4.82 s          | 4.36 s                        | 6.57 s                          | 4.82 s                        |
| 8                         | 1.48 s      | 1.76 s        | 1.58 s       | 1.74 s         | 1.43 s        | 1.46 s          | 1.39 s                        | 1.22 s                          | 1.41 s                        |
| 9                         | 338 ms      | 592 ms        | 370 ms       | 608 ms         | 333 ms        | 547 ms          | 330 ms                        | 516 ms                          | 368 ms                        |
| $\text{CHDBrI}^+$         |             |               |              |                |               |                 |                               |                                 |                               |
| 1                         | 16 min      | 16.5 min      | 17.9 min     | 20.4 min       | 8.17 min      | 9.3 min         | 2.9 min                       | 3.26 min                        | 1.37 min                      |
| 2                         | 2.79 s      | 2.75 s        | 2.73 s       | 2.71 s         | 2.16 s        | 2.16 s          | 1.65 s                        | 1.63 s                          | 1.33 s                        |
| 3                         | 3.84 s      | 3.74 s        | 3.67 s       | 3.66 s         | 3.49 s        | 3.48 s          | 3.41 s                        | 3.63 s                          | 3.21 s                        |
| 4                         | 8.93 s      | 9.3 s         | 9.12 s       | 9.57 s         | 8.46 s        | 8.67 s          | 6.73 s                        | 5.71 s                          | 6.94 s                        |
| 5                         | 9.04 s      | 11.5 s        | 9.07 s       | 10.7 s         | 9.7 s         | 11.2 s          | 7.33 s                        | 8.68 s                          | 6.15 s                        |
| 6                         | 7.05 s      | 9.29 s        | 6.33 s       | 8.86 s         | 7.04 s        | 9.11 s          | 8.24 s                        | 9.99 s                          | 8.79 s                        |
| 7                         | 5.39 s      | 6.01 s        | 5.17 s       | 5.99 s         | 3.76 s        | 4.57 s          | 3.75 s                        | 3.96 s                          | 2.75 s                        |
| 8                         | 182 ms      | 230 ms        | 194 ms       | 251 ms         | 184 ms        | 233 ms          | 172 ms                        | 211 ms                          | 191 ms                        |
| 9                         | 36.7 ms     | 47.2 ms       | 38.4 ms      | 50.2 ms        | 36.1 ms       | 46.3 ms         | 34.4 ms                       | 43.2 ms                         | 37.3 ms                       |

Table S5: Overtone ( $0 \rightarrow 2$ ) anharmonic frequencies (in  $\text{cm}^{-1}$ ) and corresponding intensities (in  $\text{km/mol}$ ) for the molecules  $\text{CH}_2\text{BrI}$ ,  $\text{CH}_2\text{BrI}^+$ ,  $\text{CHDBrI}$ , and  $\text{CHDBrI}^+$  obtained from a 3-mode analysis.

| Mode                      | PBE<br>freq | PBE<br>int | PB86<br>freq | PB86<br>int | B3LYP<br>freq | B3LYP<br>int | $\omega\text{B97X-D}$<br>freq | $\omega\text{B97X-D}$<br>int |
|---------------------------|-------------|------------|--------------|-------------|---------------|--------------|-------------------------------|------------------------------|
| $\text{CH}_2\text{BrI}$   |             |            |              |             |               |              |                               |                              |
| 1                         | 271.8       | 0.001      | 273.0        | 0.000       | 286.4         | 0.000        | 285.9                         | 0.001                        |
| 2                         | 992.1       | 0.193      | 979.1        | 0.224       | 1004.4        | 0.133        | 1065.5                        | 0.055                        |
| 3                         | 1154.7      | 0.404      | 1135.6       | 0.420       | 1178.0        | 0.355        | 1278.3                        | 0.177                        |
| 4                         | 1464.8      | 0.010      | 1464.5       | 0.008       | 1515.6        | 0.010        | 1537.5                        | 0.013                        |
| 5                         | 2055.9      | 0.102      | 2051.3       | 0.092       | 2139.9        | 0.072        | 2148.8                        | 0.081                        |
| 6                         | 2207.1      | 0.766      | 2208.9       | 0.763       | 2311.7        | 0.645        | 2314.8                        | 0.545                        |
| 7                         | 2643.8      | 0.000      | 2644.2       | 0.000       | 2757.1        | 0.005        | 2790.8                        | 0.014                        |
| 8                         | 5809.8      | 0.616      | 5790.4       | 0.604       | 5962.1        | 0.556        | 5827.6                        | 0.446                        |
| 9                         | 5934.9      | 1.219      | 5918.4       | 1.221       | 6085.8        | 1.176        | 5944.0                        | 0.968                        |
| $\text{CH}_2\text{BrI}^+$ |             |            |              |             |               |              |                               |                              |
| 1                         | 269.6       | 0.001      | 277.1        | 0.001       | 256.5         | 0.001        | 318.7                         | 0.003                        |
| 2                         | 974.3       | 0.010      | 958.7        | 0.007       | 963.9         | 0.011        | 1061.8                        | 0.033                        |
| 3                         | 1162.0      | 0.042      | 1158.7       | 0.045       | 1170.9        | 0.065        | 1268.7                        | 0.068                        |
| 4                         | 1583.6      | 0.027      | 1578.0       | 0.027       | 1628.2        | 0.033        | 1651.2                        | 0.037                        |
| 5                         | 1922.3      | 0.115      | 1927.1       | 0.104       | 1991.3        | 0.086        | 2057.5                        | 0.106                        |
| 6                         | 2143.3      | 0.996      | 2152.3       | 1.003       | 2234.0        | 0.879        | 2290.2                        | 0.830                        |
| 7                         | 2635.9      | 0.140      | 2641.2       | 0.144       | 2741.6        | 0.140        | 2777.5                        | 0.139                        |
| 8                         | 5806.2      | 0.671      | 5794.1       | 0.665       | 5961.6        | 0.591        | 5927.2                        | 0.492                        |
| 9                         | 5990.1      | 1.111      | 5974.5       | 1.114       | 6137.9        | 1.032        | 6094.8                        | 0.870                        |
| $\text{CHDBrI}$           |             |            |              |             |               |              |                               |                              |
| 1                         | 258.0       | 0.001      | 258.7        | 0.000       | 279.5         | 0.000        | 261.7                         | 0.000                        |
| 2                         | 950.6       | 0.134      | 946.5        | 0.165       | 970.9         | 0.107        | 1023.0                        | 0.038                        |
| 3                         | 1120.6      | 0.420      | 1107.4       | 0.520       | 1145.7        | 0.458        | 1227.5                        | 0.235                        |
| 4                         | 1254.7      | 0.169      | 1258.3       | 0.177       | 1302.7        | 0.212        | 1317.5                        | 0.177                        |
| 5                         | 1535.4      | 0.182      | 1541.3       | 0.174       | 1612.0        | 0.141        | 1623.7                        | 0.133                        |
| 6                         | 2115.6      | 0.616      | 2123.4       | 0.590       | 2221.2        | 0.405        | 2211.2                        | 0.096                        |
| 7                         | 2357.1      | 0.252      | 2361.8       | 0.240       | 2460.2        | 0.229        | 2485.3                        | 0.234                        |
| 8                         | 4339.3      | 0.635      | 4328.8       | 0.628       | 4454.6        | 0.603        | 4363.9                        | 0.498                        |
| 9                         | 5809.7      | 1.569      | 5791.4       | 1.558       | 5964.1        | 1.496        | 5799.0                        | 1.213                        |
| $\text{CHDBrI}^+$         |             |            |              |             |               |              |                               |                              |
| 1                         | 271.8       | 0.001      | 256.3        | 0.001       | 261.7         | 0.000        | 296.9                         | 0.003                        |
| 2                         | 952.1       | 0.010      | 931.0        | 0.005       | 942.6         | 0.005        | 1026.5                        | 0.025                        |
| 3                         | 1134.9      | 0.045      | 1114.1       | 0.046       | 1137.6        | 0.066        | 1210.0                        | 0.068                        |
| 4                         | 1337.1      | 0.126      | 1326.7       | 0.127       | 1378.8        | 0.137        | 1399.7                        | 0.126                        |
| 5                         | 1484.0      | 0.181      | 1470.8       | 0.173       | 1532.7        | 0.155        | 1571.2                        | 0.165                        |
| 6                         | 2051.3      | 1.003      | 2044.0       | 0.984       | 2137.4        | 0.889        | 2173.7                        | 0.896                        |
| 7                         | 2367.1      | 0.732      | 2362.2       | 0.702       | 2456.9        | 0.670        | 2483.3                        | 0.680                        |
| 8                         | 4362.1      | 0.529      | 4346.8       | 0.525       | 4471.9        | 0.480        | 4445.4                        | 0.402                        |
| 9                         | 5849.8      | 1.368      | 5829.8       | 1.366       | 6000.1        | 1.250        | 5938.9                        | 1.036                        |

### S3. Dependence of the PV energy shift on the level of theory

The CH wagging mode (mode 6) in CHDBrI<sup>+</sup> turns out to be a very promising candidate for future high-precision spectroscopy experiments. Therefore, to ensure the reliability of our theoretical prediction for the magnitude of the PV frequency shift  $\Delta\nu^{\text{PV}}$  for this mode, we tested the effect of the basis set applied, our computational approach (HF vs. DFT), and the choice of the functional used on our results. From Table S6, we can see that using a smaller basis set (Def2-TZVP) has only a minor effect on the PV frequency difference. Hybrid DFT functionals sit at the intersection of the delocalized LDA and localized HF. By comparing our results to these extremes, we can easily set very conservative bounds on the result without the need to test an entire spectrum of DFT functionals. HF and LDA yield significantly different values. However, the PV frequency shift is still in the ballpark of 1 Hz, which gives confidence for our method used, even in the case when HF was used also for the optimization step. The result can thus be considered fairly robust. We have thoroughly tested the dependence of the result on the parameters of the methodology in our previous work<sup>11</sup> with a similar conclusion.

Table S6: Calculated PV frequency shift  $\Delta\nu^{\text{PV}}$  (in Hz) for vibrational mode 6 of (R)-CHDBrI<sup>+</sup> on different levels of theory (method or functional / basis set). Reference method and result shown in bold.

| Geometry optimization                | DIRAC calculations             | $\Delta\nu^{\text{PV}}$ |
|--------------------------------------|--------------------------------|-------------------------|
| $\omega$ <b>B97M-V / Def2-QZVPPD</b> | <b>CAM-B3LYP* / Dyall.av4z</b> | <b>-1.78</b>            |
| $\omega$ B97M-V / Def2-TZVP          | CAM-B3LYP* / Dyall.v3z         | -1.72                   |
| $\omega$ B97M-V / Def2-QZVPPD        | HF / Dyall.av4z                | -1.37                   |
| $\omega$ B97M-V / Def2-QZVPPD        | LDA / Dyall.av4z               | -0.86                   |
| HF / Def2-QZVPPD                     | HF / Dyall.av4z                | -0.86                   |

# S4. Orbital contributions analysis for mode 6 of CHD-BrI and CHDBrI<sup>+</sup>

Figure S1 presents the atomic contributions to the total PV energy difference for mode 6 of CHDBrI and CHDBrI<sup>+</sup>. For both species, the bromine and iodine contributions dominate over the lighter atoms, but we observe a very different behaviour of the two molecules for mode 6. For the cation, the shape of the PV curve exhibits a strong curvature, while for the neutral molecule we see an almost linear behaviour (for the total as well as atomic PV contributions). The latter leads to a very small PV vibrational frequency shift as the second derivative  $\partial^2 E^{\text{PV}}/\partial q^2(q = 0)$  becomes zero (or close to zero). To understand this different behaviour we further consider the individual molecular orbital (MO) contributions of the two atoms Br and I contributing most to the PV energy shift.

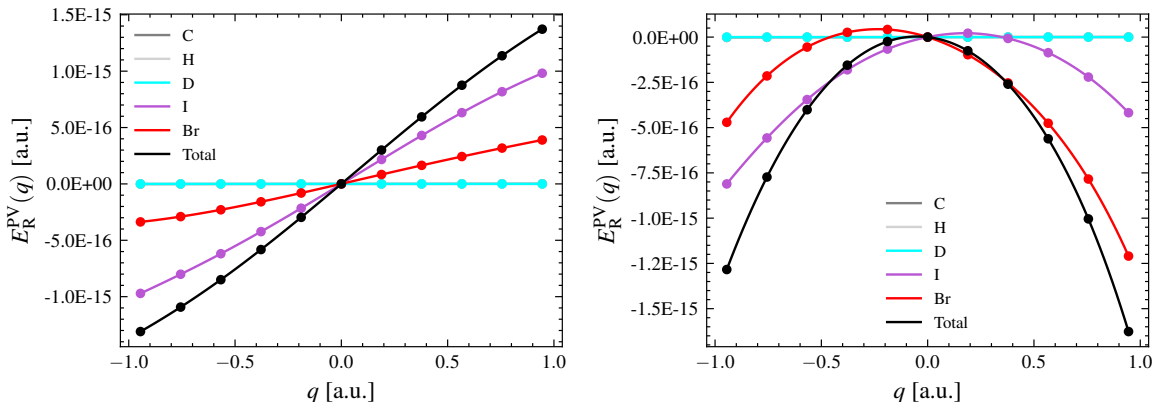

Figure S1: Breakdown of the atomic contributions to the total PV energy  $E^{\text{PV}}(q)$  along mode 6 in (R)-CHDBrI (left) and (R)-CHDBrI<sup>+</sup> (right).

There are in total 48 occupied MOs in our calculations for CHDBrI (note that a pseudopotential was used for the iodine atom). Analysis of the added orbital contributions from the 47 orbitals up to and including HOMO – 1 is shown in Figure S2. For both CHDBrI and

CHDBrI<sup>+</sup> we observe, for the PV contributions up to and including HOMO – 1, an almost even PV curve of (approximately) second order in  $q$  with bromine being the main contributor to the PV. However, the HOMO orbital contribution shown in Figure S2 changes the shape of the total PV curve to an odd function of (approximately) third order in  $q$  for the neutral molecule, in contrast to the cationic species. Based on this analysis, it is clear that the removal of a HOMO electron in the neutral molecule makes the contribution from the inner orbitals dominant, which translates into an even function that has a strong curvature. Further support of this argument can be seen from the bottom panels in Figure S2, where the doubling of the HOMO contribution in the cation (artificial addition of 1 electron) results in an approximately odd PV function resembling the neutral molecule. Similarly, halving the HOMO contribution in the neutral system (artificial removal of 1 electron) results in an approximately even function of the PV curve resembling the unaltered cation.

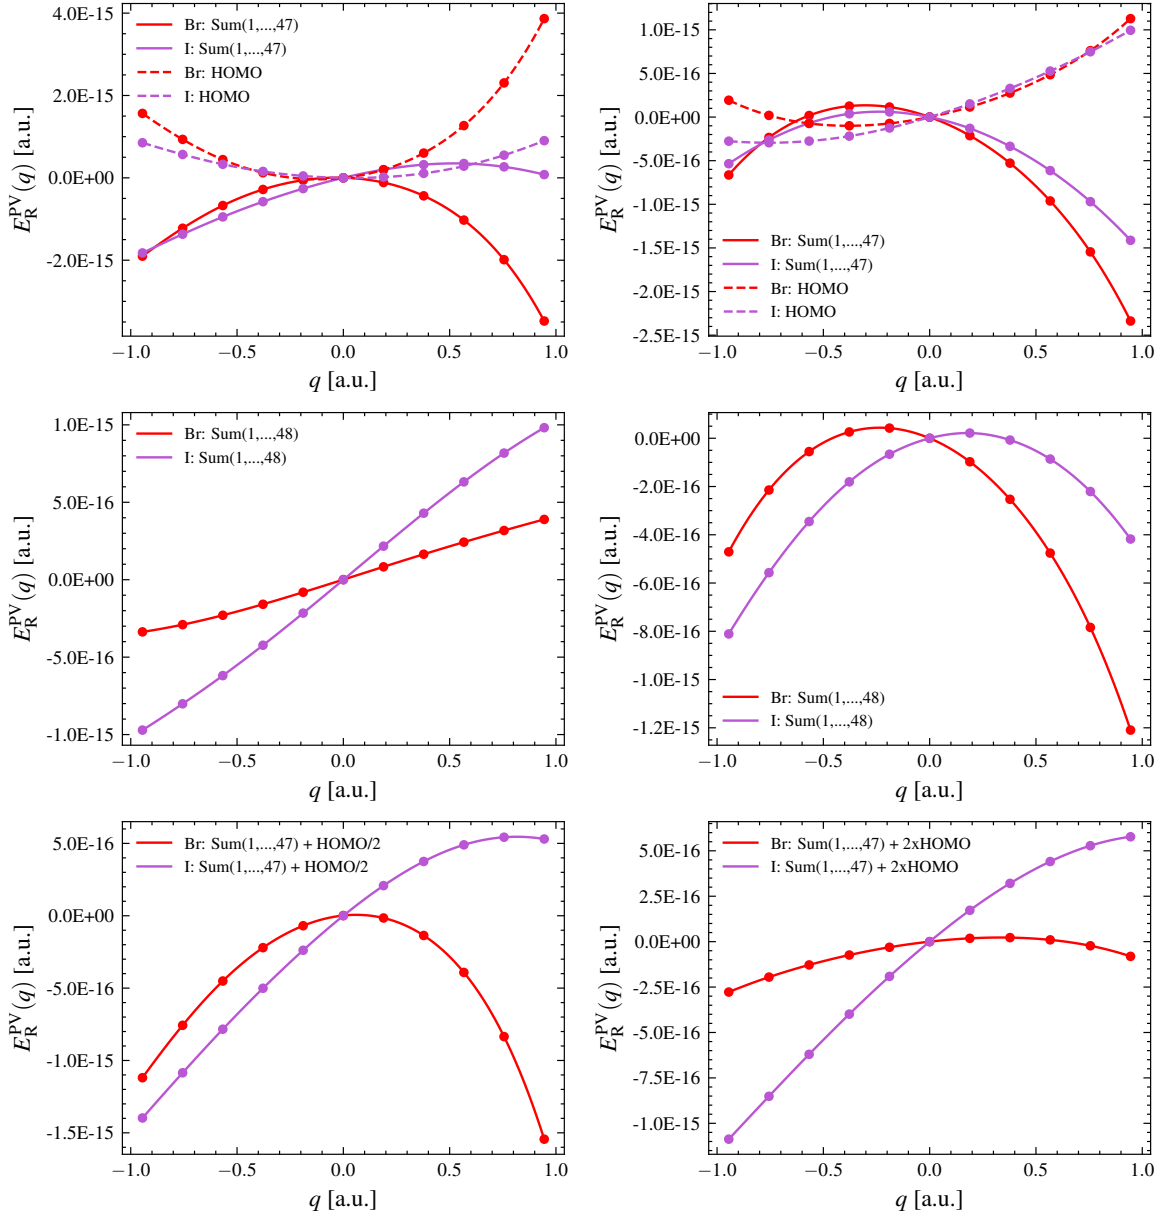

Figure S2: Orbital contributions of PV energies  $E^{\text{PV}}(q)$  along mode 6 in the neutral (left) and cation (right) of (R)-CHDBrI. Top: Added PV contributions up to and including the HOMO – 1 orbital (MO 47) and separate HOMO (MO 48) contribution. Middle: Added PV contributions up to and including MO 48 (HOMO). Bottom: Artificial electron removal/addition in (R)-CHDBrI/(R)-CHDBrI<sup>+</sup> (left/right panel) by means of halving/doubling the HOMO (MO 48) contribution.

## S5. Additional Information

Table S6 shows the results of the VPT analysis of the PV energies for all modes. Mode 6 was discussed in the main text. Similarly, modes 5 and 7 are dominated by the harmonic VPT term. In contrast, modes 8 and 9 corresponding to the H/D stretching, which are strongly anharmonic, are dominated by the anharmonic VPT term.

Figure S3 summarizes potential energy  $V(q)$  and PV  $E^{\text{PV}}(q)$  curves for all modes of both molecules. This visually supports the VPT analysis in Figures S4.

Finally, Figures S4–S11 show orbital decomposition analysis for modes 1–5 and 7–9 analogous to that of mode 6 shown on Figure S2 and discussed in the previous section. Similar cancellation effects (and their reduction in the ionized molecule) can be observed for these modes.

Table S7: PV value for Numerov–Cooley (NC) procedure and VPT (vibrational perturbation theory) values  $\Delta\nu^{\text{PV}}$  (in Hz) for (R)-CHDBrI<sup>+</sup>. Curvature and anharmonic VPT contributions are shown separately (refer to Eq. (2) in the main text).

| Mode<br>number | CHDBrI  |         |           |             | CHDBrI <sup>+</sup> |         |           |             |
|----------------|---------|---------|-----------|-------------|---------------------|---------|-----------|-------------|
|                | NC      | VPT     | VPT curv. | VPT anharm. | NC                  | VPT     | VPT curv. | VPT anharm. |
| 1              | −0.0010 | −0.0010 | −0.0006   | 0.0004      | 0.0088              | 0.0088  | 0.0054    | −0.0035     |
| 2              | −0.0442 | −0.0423 | −0.0346   | 0.0078      | −0.1256             | −0.1145 | −0.0373   | 0.0772      |
| 3              | 0.2419  | 0.2347  | 0.0860    | −0.1487     | −0.0367             | −0.0457 | 0.2489    | 0.2946      |
| 4              | −0.0509 | −0.0523 | −0.0567   | −0.0044     | −0.0415             | −0.0769 | −0.0321   | 0.0448      |
| 5              | −0.0614 | −0.0649 | −0.0490   | 0.0159      | 1.3352              | 1.3452  | 1.3264    | −0.0188     |
| 6              | 0.0534  | 0.0292  | 0.0493    | 0.0200      | −1.7789             | −1.8421 | −1.8405   | 0.0016      |
| 7              | 0.0428  | 0.0535  | 0.0203    | −0.0332     | −0.5901             | −0.6102 | −0.5573   | 0.0529      |
| 8              | 0.0177  | 0.0194  | 0.0155    | −0.0039     | 0.9370              | 0.8541  | 0.2086    | −0.6454     |
| 9              | −0.0549 | −0.0555 | −0.0022   | 0.0533      | −1.2918             | −1.1562 | −0.2159   | 0.9403      |

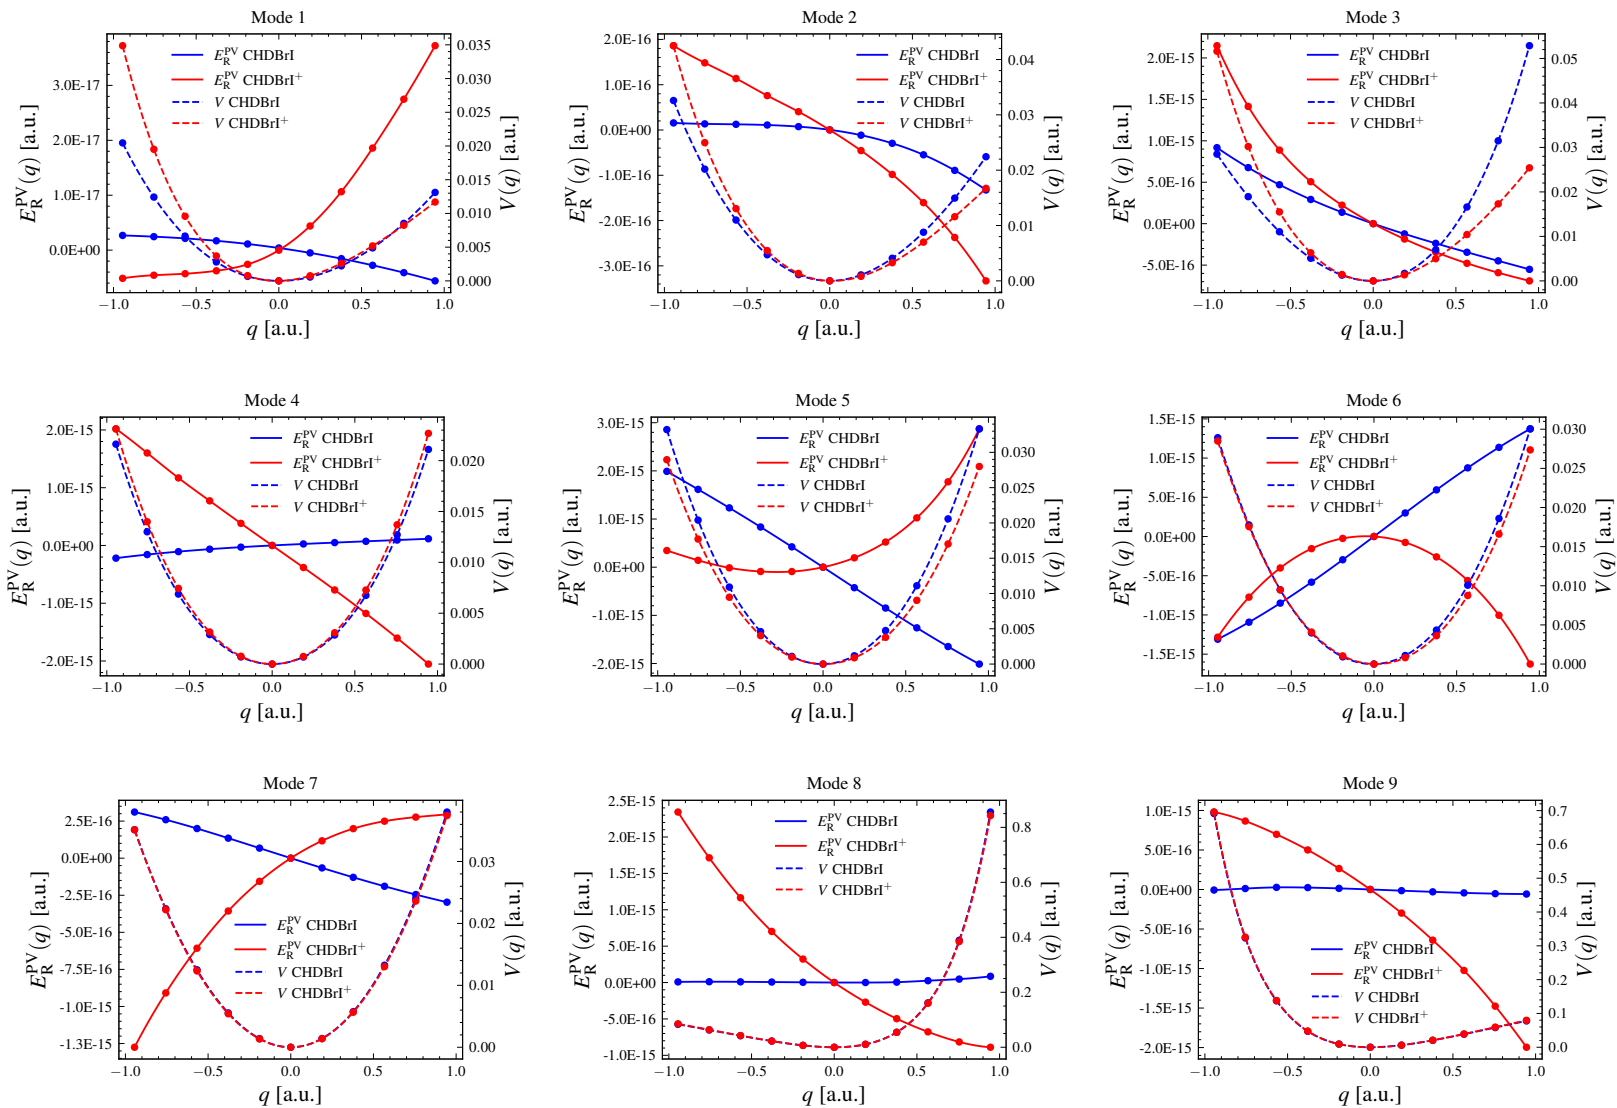

Figure S3: Comparison between (R)-CHDBrI and (R)-CHDBrI<sup>+</sup> for the potential energy  $V(q)$  and PV  $E^{PV}(q)$  curves.

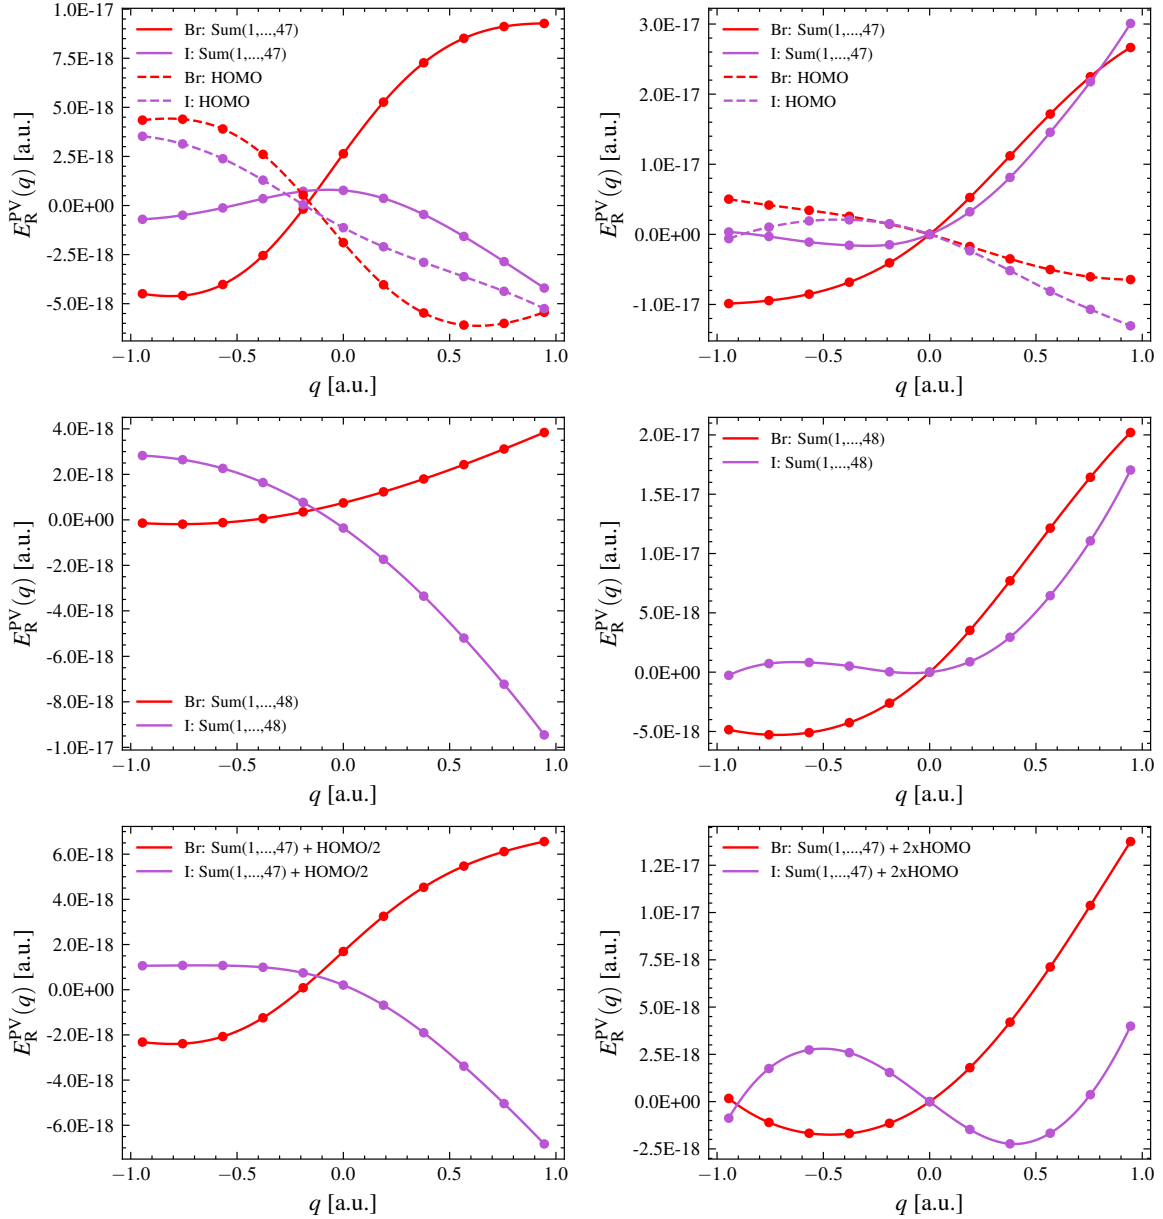

Figure S4: Orbital contributions of PV energies  $E^{\text{PV}}(q)$  along mode 1 in the neutral (left) and cation (right) of (R)-CHDBrI. Top: Added PV contributions up to and including the HOMO – 1 orbital (MO 47) and separate HOMO (MO 48) contribution. Middle: Added PV contributions up to and including MO 48 (HOMO). Bottom: Artificial electron removal/addition in (R)-CHDBrI/(R)-CHDBrI<sup>+</sup> (left/right panel) by means of halving/doubling the HOMO (MO 48) contribution.

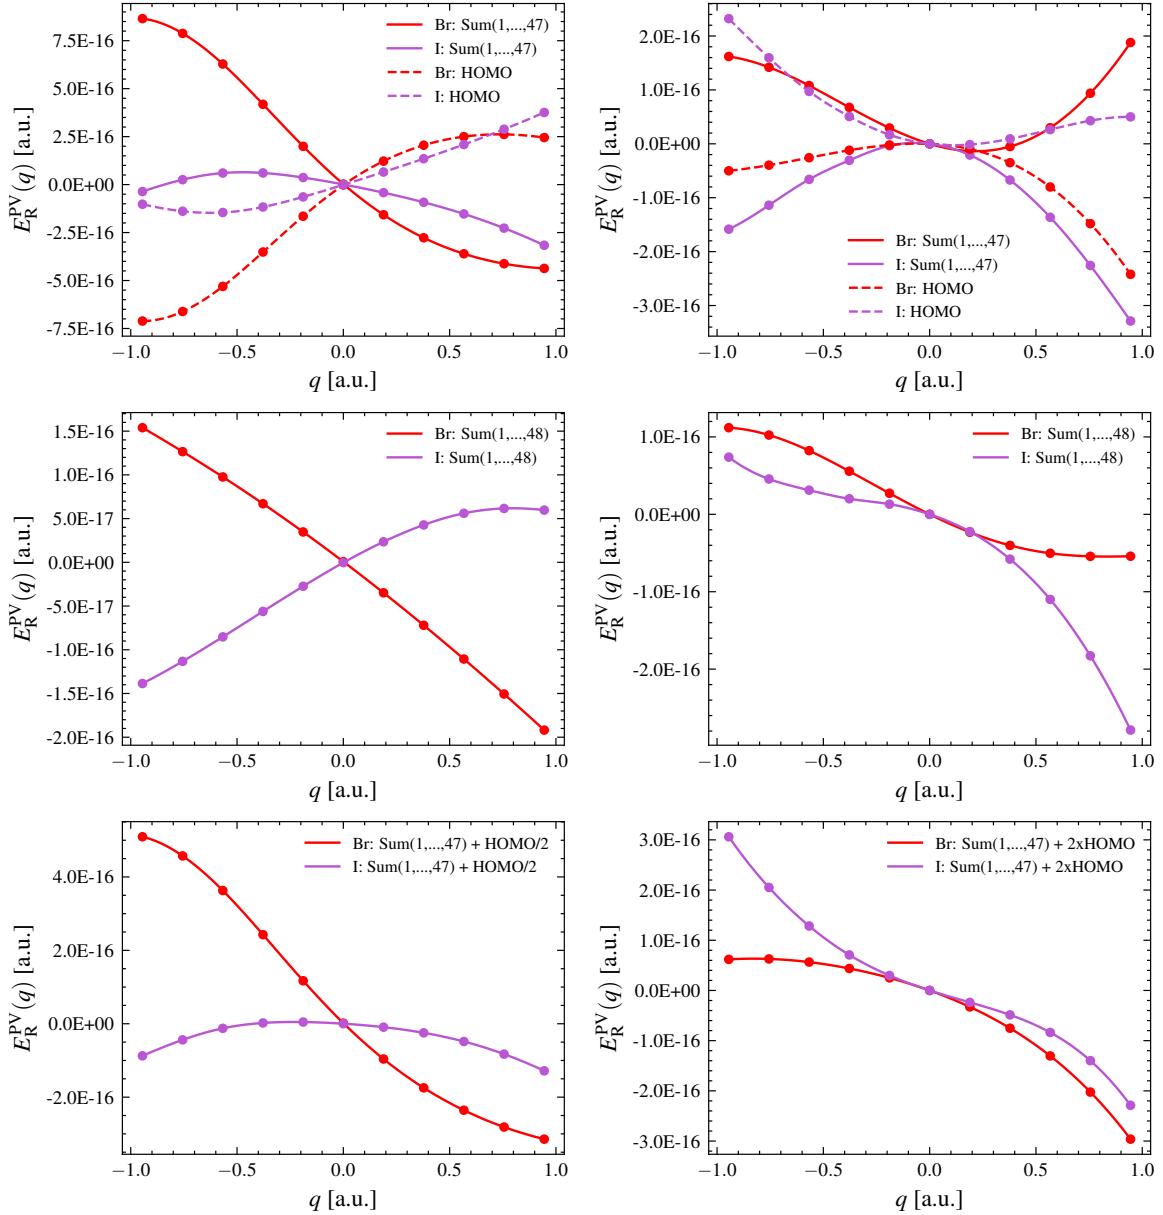

Figure S5: Orbital contributions of PV energies  $E^{\text{PV}}(q)$  along mode 2 in the neutral (left) and cation (right) of (R)-CHDBrI. Top: Added PV contributions up to and including the HOMO – 1 orbital (MO 47) and separate HOMO (MO 48) contribution. Middle: Added PV contributions up to and including MO 48 (HOMO). Bottom: Artificial electron removal/addition in (R)-CHDBrI/(R)-CHDBrI<sup>+</sup> (left/right panel) by means of halving/doubling the HOMO (MO 48) contribution.

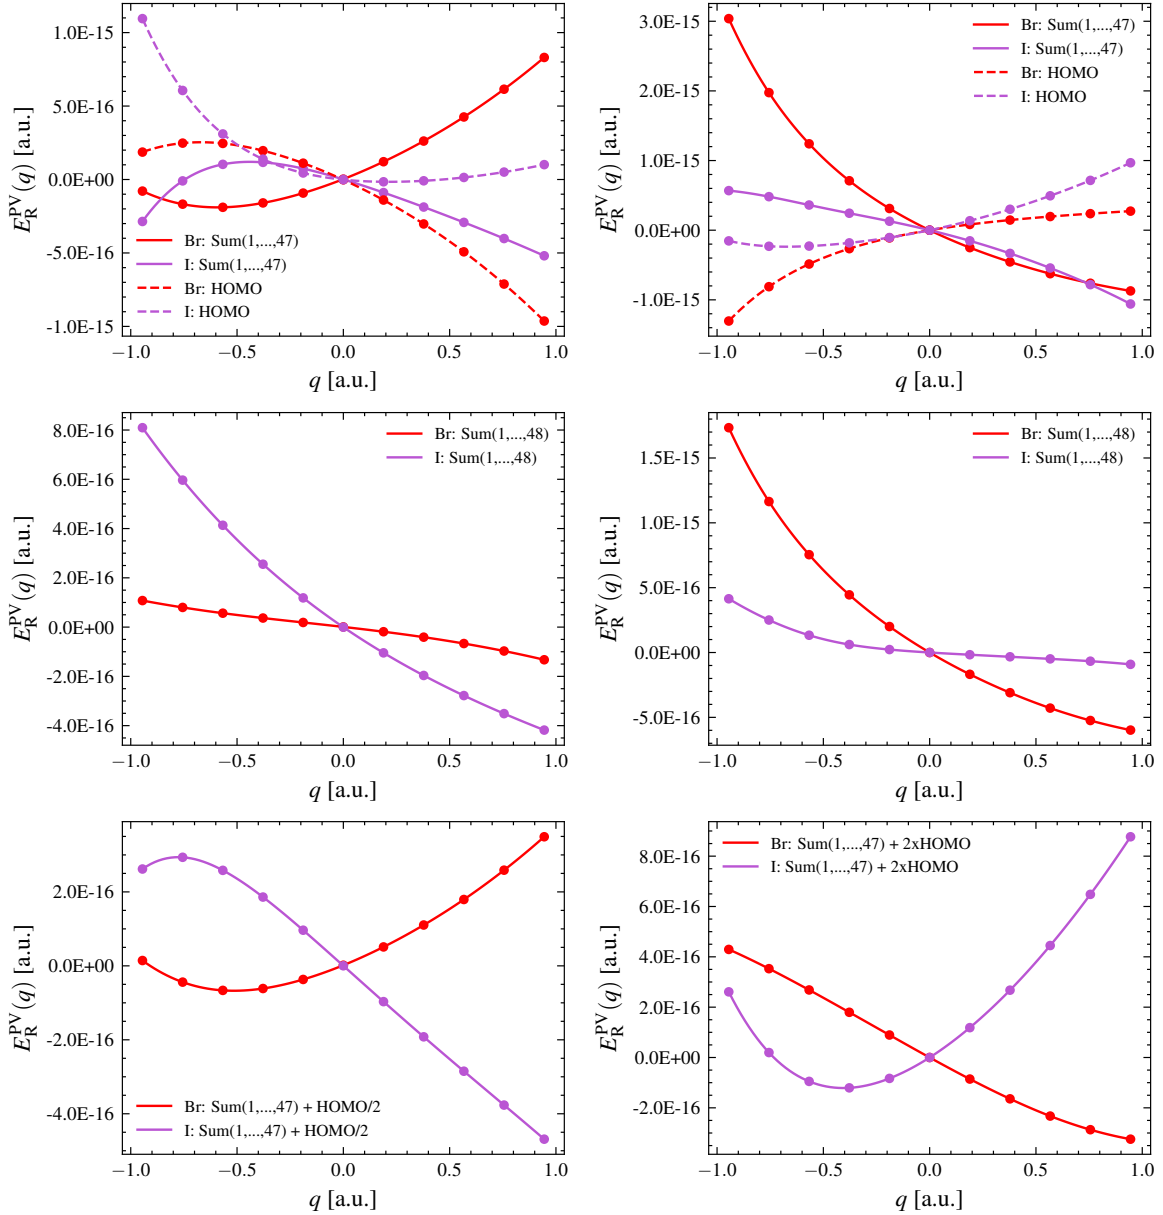

Figure S6: Orbital contributions of PV energies  $E^{PV}(q)$  along mode 3 in the neutral (left) and cation (right) of (R)-CHDBrI. Top: Added PV contributions up to and including the HOMO – 1 orbital (MO 47) and separate HOMO (MO 48) contribution. Middle: Added PV contributions up to and including MO 48 (HOMO). Bottom: Artificial electron removal/addition in (R)-CHDBrI/(R)-CHDBrI<sup>+</sup> (left/right panel) by means of halving/doubling the HOMO (MO 48) contribution.

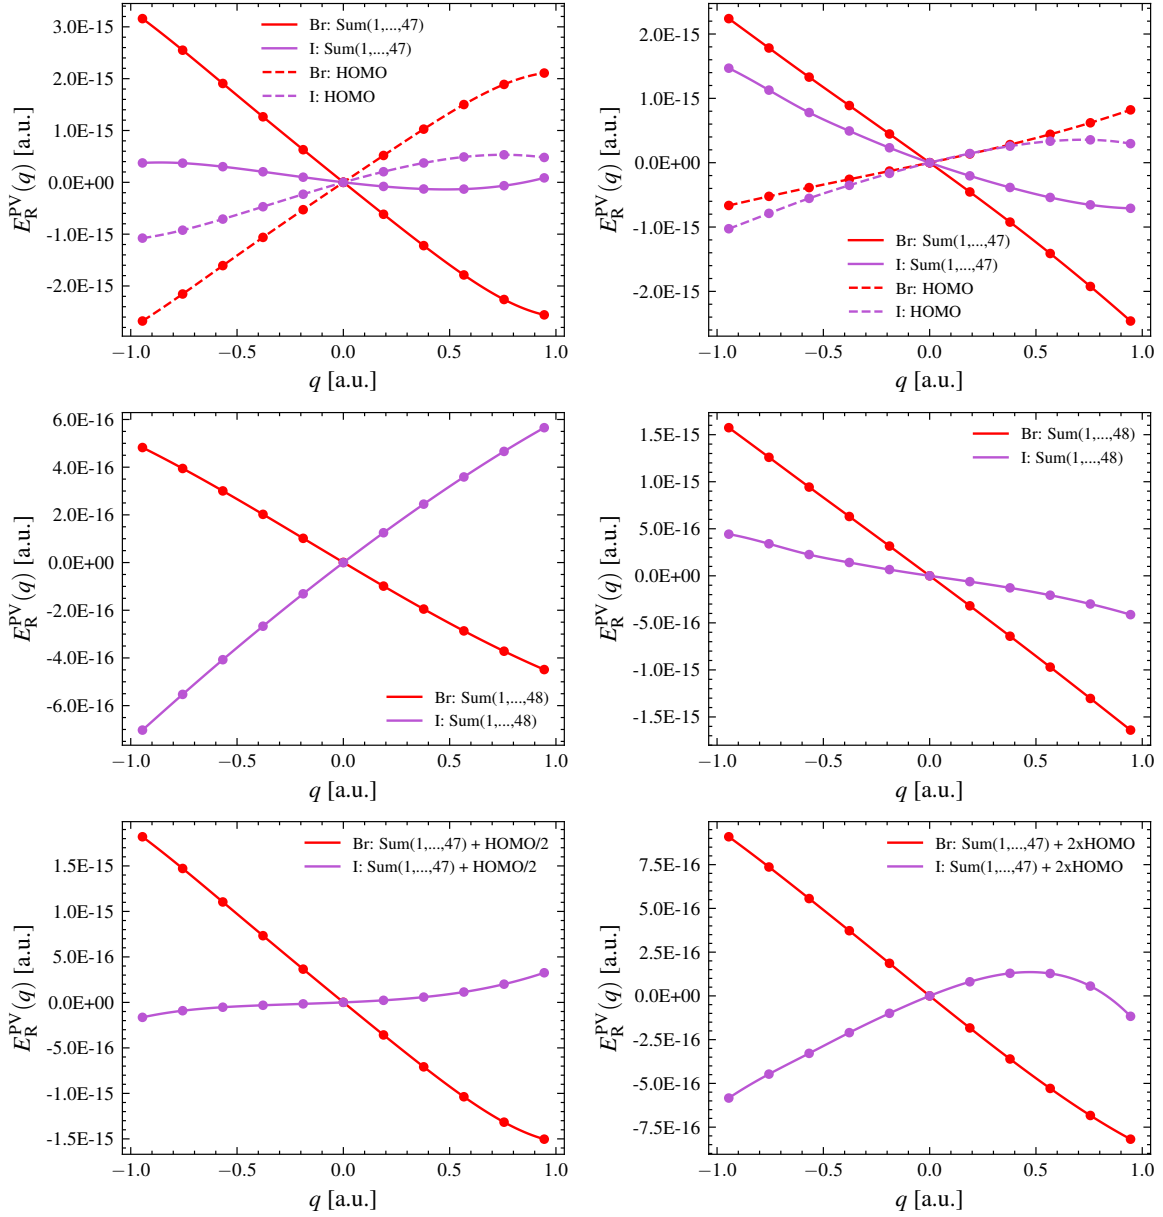

Figure S7: Orbital contributions of PV energies  $E^{\text{PV}}(q)$  along mode 4 in the neutral (left) and cation (right) of (R)-CHDBrI. Top: Added PV contributions up to and including the HOMO – 1 orbital (MO 47) and separate HOMO (MO 48) contribution. Middle: Added PV contributions up to and including MO 48 (HOMO). Bottom: Artificial electron removal/addition in (R)-CHDBrI/(R)-CHDBrI<sup>+</sup> (left/right panel) by means of halving/doubling the HOMO (MO 48) contribution.

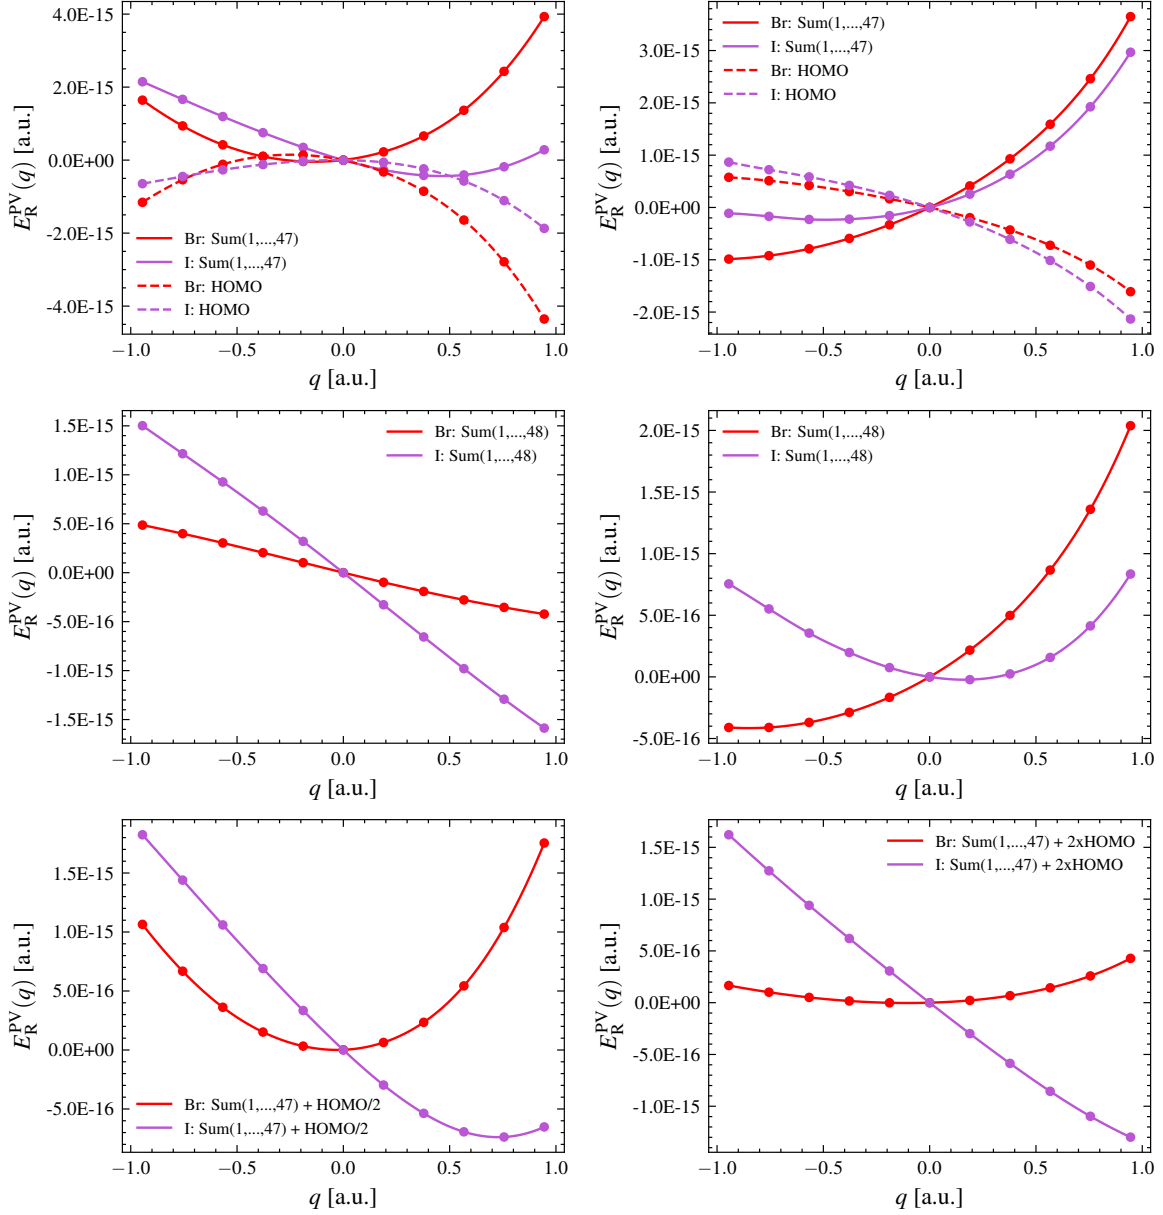

Figure S8: Orbital contributions of PV energies  $E^{PV}(q)$  along mode 5 in the neutral (left) and cation (right) of (R)-CHDBrI. Top: Added PV contributions up to and including the HOMO – 1 orbital (MO 47) and separate HOMO (MO 48) contribution. Middle: Added PV contributions up to and including MO 48 (HOMO). Bottom: Artificial electron removal/addition in (R)-CHDBrI/(R)-CHDBrI<sup>+</sup> (left/right panel) by means of halving/doubling the HOMO (MO 48) contribution.

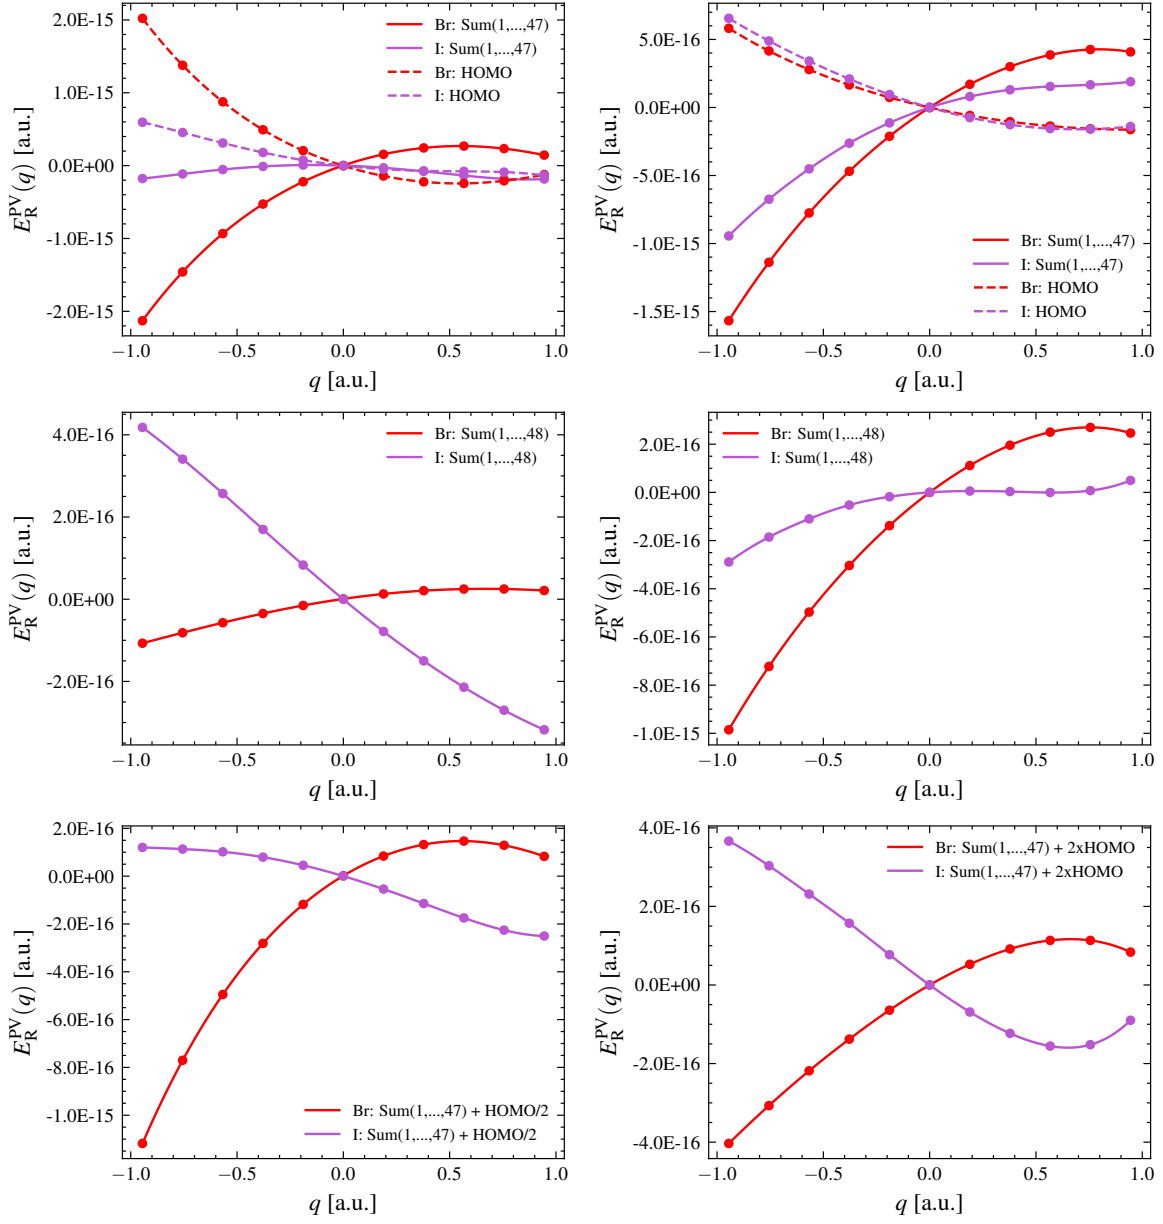

Figure S9: Orbital contributions of PV energies  $E_R^{PV}(q)$  along mode 7 in the neutral (left) and cation (right) of (R)-CHDBrI. Top: Added PV contributions up to and including the HOMO – 1 orbital (MO 47) and separate HOMO (MO 48) contribution. Middle: Added PV contributions up to and including MO 48 (HOMO). Bottom: Artificial electron removal/addition in (R)-CHDBrI/(R)-CHDBrI<sup>+</sup> (left/right panel) by means of halving/doubling the HOMO (MO 48) contribution.

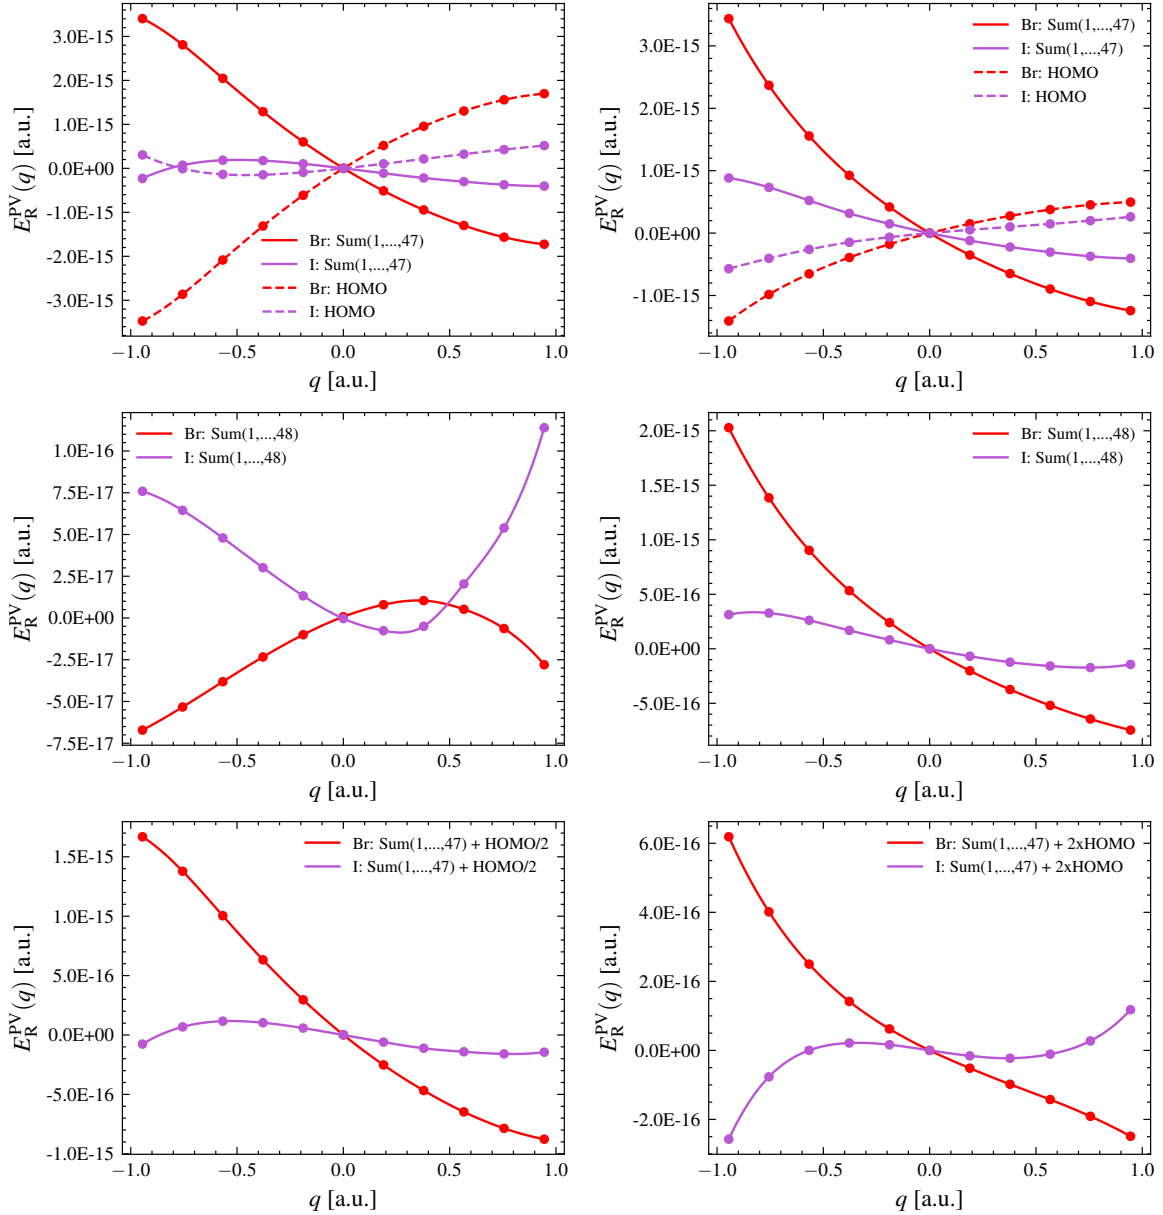

Figure S10: Orbital contributions of PV energies  $E^{PV}(q)$  along mode 8 in the neutral (left) and cation (right) of (R)-CHDBrI. Top: Added PV contributions up to and including the HOMO – 1 orbital (MO 47) and separate HOMO (MO 48) contribution. Middle: Added PV contributions up to and including MO 48 (HOMO). Bottom: Artificial electron removal/addition in (R)-CHDBrI/(R)-CHDBrI<sup>+</sup> (left/right panel) by means of halving/doubling the HOMO (MO 48) contribution.

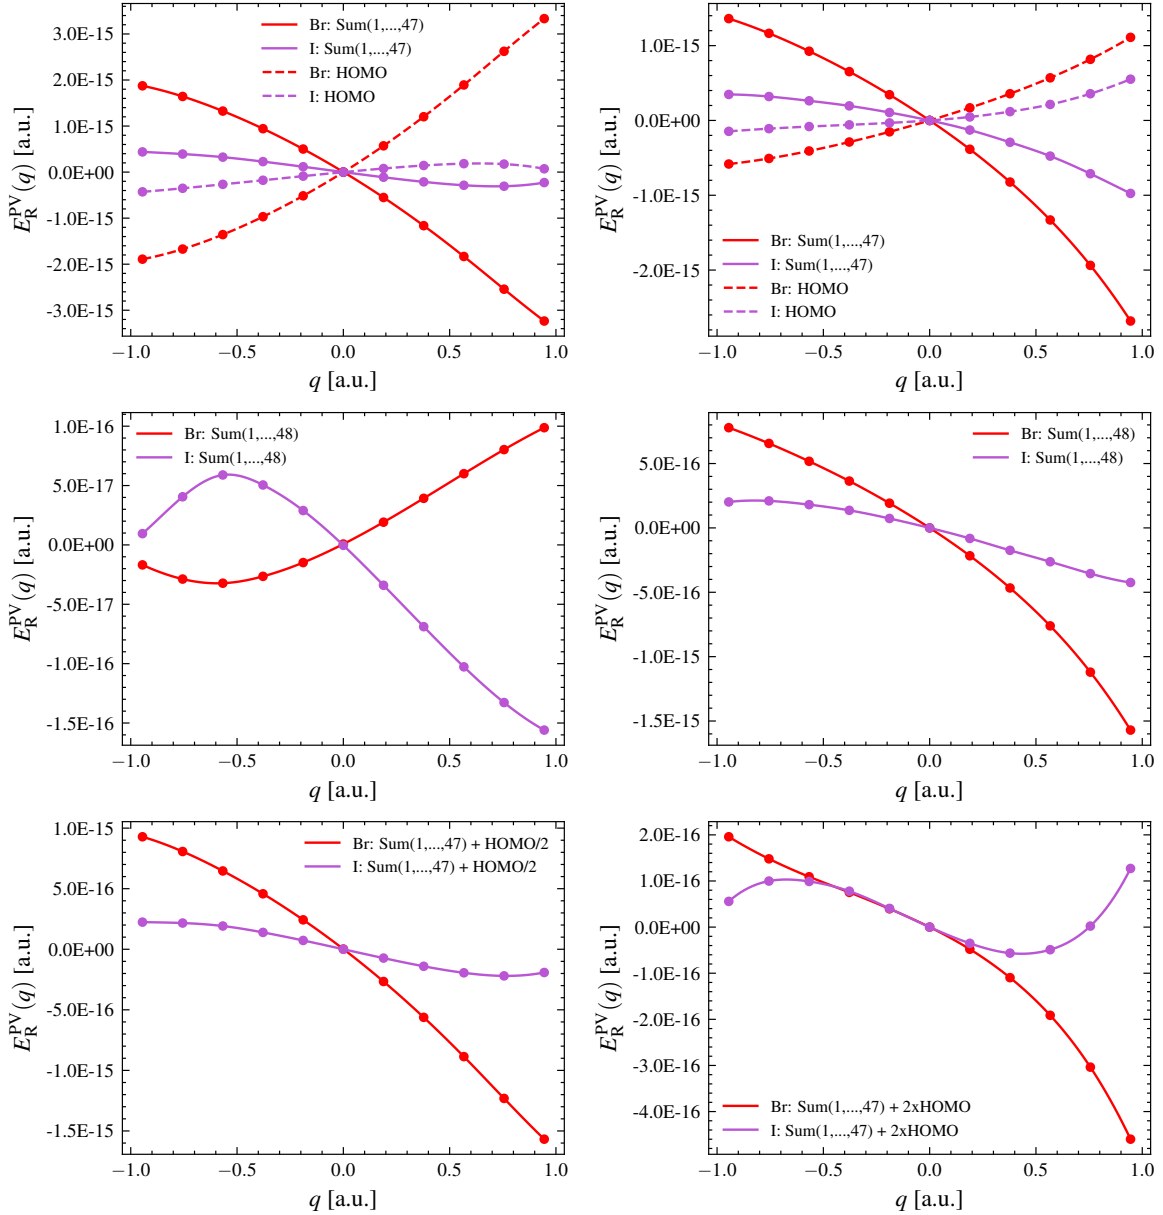

Figure S11: Orbital contributions of PV energies  $E^{\text{PV}}(q)$  along mode 9 in the neutral (left) and cation (right) of (R)-CHDBrI. Top: Added PV contributions up to and including the HOMO – 1 orbital (MO 47) and separate HOMO (MO 48) contribution. Middle: Added PV contributions up to and including MO 48 (HOMO). Bottom: Artificial electron removal/addition in (R)-CHDBrI/(R)-CHDBrI<sup>+</sup> (left/right panel) by means of halving/doubling the HOMO (MO 48) contribution.

## References

- (1) Clabo, D.; Allen, W. D.; Remington, R. B.; Yamaguchi, Y.; Schaefer, H. F. A systematic study of molecular vibrational anharmonicity and vibration—rotation interaction by self-consistent-field higher-derivative methods. Asymmetric top molecules. *Chemical Physics* **1988**, *123*, 187–239.
- (2) Barone, V. Anharmonic vibrational properties by a fully automated second-order perturbative approach. *The Journal of Chemical Physics* **2004**, *122*, 014108.
- (3) Carbonniere, P.; Lucca, T.; Pouchan, C.; Rega, N.; Barone, V. Vibrational computations beyond the harmonic approximation: Performances of the B3LYP density functional for semirigid molecules. *Journal of Computational Chemistry* **2005**, *26*, 384–388.
- (4) Rauhut, G.; Barone, V.; Schwerdtfeger, P. Vibrational analyses for CHFCIBr and CDFClBr based on high level *ab initio* calculations. *The Journal of Chemical Physics* **2006**, *125*, 054308.
- (5) Thierfelder, C.; Rauhut, G.; Schwerdtfeger, P. Relativistic coupled-cluster study of the parity-violation energy shift of CHFCIBr. *Physical Review A* **2010**, *81*, 032513.
- (6) Rappoport, D.; Furche, F. Property-optimized Gaussian basis sets for molecular response calculations. *The Journal of Chemical Physics* **2010**, *133*, 134105.
- (7) Mardirossian, N.; Head-Gordon, M.  $\omega$ B97M-V: A combinatorially optimized, range-separated hybrid, meta-GGA density functional with VV10 nonlocal correlation. *The Journal of Chemical Physics* **2016**, *144*, 214110.
- (8) Bailleux, S.; Duflot, D.; Taniguchi, K.; Sakai, S.; Ozeki, H.; Okabayashi, T.; Bailey, W. C. Fourier Transform Microwave and Millimeter-Wave Spectroscopy of Bromiodomethane, CH<sub>2</sub>BrI. *The Journal of Physical Chemistry A* **2014**, *118*, 11744–11750.

- (9) El-Sabban, M. Z.; Danti, A.; Zwolinski, B. J. Normal-Coordinate Analysis and Molecular Properties of Four  $\text{CH}_2\text{XY}$  Halomethanes ( $\text{X} = \text{F}$  or  $\text{I}$ ;  $\text{Y} = \text{Cl}$  or  $\text{Br}$ ). *The Journal of Chemical Physics* **1966**, *44*, 1770–1779.
- (10) Wu, T. Systematics in the Vibrational Spectra of the Halogen Derivatives of Methane. *The Journal of Chemical Physics* **2004**, *10*, 116–124.
- (11) Fiechter, M. R.; Haase, P. A. B.; Saleh, N.; Soulard, P.; Tremblay, B.; Havenith, R. W. A.; Timmermans, R. G. E.; Schwerdtfeger, P.; Crassous, J.; Darquié, B.; Pašteka, L. F.; Borschevsky, A. Toward Detection of the Molecular Parity Violation in Chiral  $\text{Ru}(\text{acac})_3$  and  $\text{Os}(\text{acac})_3$ . *The Journal of Physical Chemistry Letters* **2022**, *13*, 10011–10017.
